# Supplementary material for: BEA: Revisiting anchor-based object detection DNN using Budding Ensemble Architecture
Source: arXiv:2309.08036 source file (2023-11-10)
Supplement: Supplementary file 1 [file suppl_ablation_bea_div.tex]

\begin{table*}[hbt!]
\resizebox{\linewidth}{!}{
\centering
\captionsetup{justification=centering}
\begin{tabular}{|c|c|c|c|c|c|ccc|}
\hline
% \multirow{2}{*}{
\begin{tabular}[c]{@{}c@{}}BEA + $\mathcal{L_{\mbox{tandem}}}$ + $\mathcal{\lambda_{D}*L_{\mbox{Diveristy}}}$; $\lambda_{D}=1$\end{tabular}
& \multirow{2}{*}{$mAP_{raw}$ $\mathbf{\uparrow}$} & \multirow{2}{*}{$AP50_{raw}$ $\mathbf{\uparrow}$} & \multirow{2}{*}{$AP50_{\mathcal{U}_{pred}}$ $\mathbf{\uparrow}$} & \multirow{2}{*}{$UE$ (\%) $\mathbf{\downarrow}$} & \multirow{2}{*}{\begin{tabular}[c]{@{}c@{}}Retention Curve\\ $AUC$ (\%) $\mathbf{\uparrow}$\end{tabular}} & \multicolumn{3}{|c|}{\begin{tabular}[c]{@{}c@{}}Out-of-distribution detection (OOD) \\ $AUC-ROC$ (\%)$\mathbf{\uparrow}$ \end{tabular}} \\
\cline{1-1} \cline{7-9} Diversity (similarity score) &  & & & & & \multicolumn{1}{c|}{\begin{tabular}[|c|]{@{}c@{}}CityPersons \\$\mathcal{U}_{near-ood}$ \end{tabular}} & \multicolumn{1}{c|}{\begin{tabular}[c]{@{}c@{}}BDD100K\\ $\mathcal{U}_{near-ood}$\end{tabular}} & \begin{tabular}[c]{@{}c@{}}COCO\\$\mathcal{U}_{far-ood}$\end{tabular} \\ \hline
linearCKA       &  54.63 & 88.76 &  85.84 & 4.41 & 74.5 & \multicolumn{1}{c|}{93.51} & \multicolumn{1}{c|}{87.26} & 97.36  \\ \hline
column-wise &  53.2  & 88.44 &  84.61 & 4.43 & 73.7 & \multicolumn{1}{c|}{85.32} & \multicolumn{1}{c|}{87.42} & 97.56  \\ \hline
row-wise        &  53.35 & 89.07  & 84.69 & 4.81 & 74.8 & \multicolumn{1}{c|}{80.97} & \multicolumn{1}{c|}{82.35} & 96     \\ \hline
row-column wise &  52.63 &  88.5 & 84.73 &  4.64 & 73.6 & \multicolumn{1}{c|}{83.5} & \multicolumn{1}{c|}{87.3} & 96.97 \\ \hline
kernelCKA ($\sigma=0.8$) &  49.7 &  88.39 & 83.92 & 5.8 & 72.2 & \multicolumn{1}{c|}{83.8} & \multicolumn{1}{c|}{85.73} & 97.84 \\ \hline
kernelCKA ($\sigma=None$) & 49.9 &  88.09 & 83.67 & 5.24 & 74 & \multicolumn{1}{c|}{82.21} & \multicolumn{1}{c|}{85.53} & 97.08 \\ \hline
% D &  54.42 &  \textbf{89.49} & 82.23 & 8.65 & 57.5& \multicolumn{1}{c|}{TBA} & \multicolumn{1}{c|}{TBA} & TBA \\ \hline
% D &  \textit{\textbf{54.63}} &  \textit{\textbf{88.76}} & \textbf{85.8} & \textbf{4.41}  & \textbf{74.5}& \multicolumn{1}{c|}{TBA} & \multicolumn{1}{c|}{TBA} & TBA \\ \hline
\end{tabular}%
}
\captionsetup{skip=\dimexpr\abovecaptionskip+3pt}
\caption{Extended Ablation study on BEA-YOLOv3 with different Diversity scores: Effects on the accuracy, uncertainty error, calibration and out-of-distribution shown by $\mathcal{L_{\mbox{tandem}}}$ and $\lambda_{D}*\mathcal{L_{\mbox{Diveristy}}}$}
\label{tab:supp_ablation_bea_div}
\end{table*}
